# Supplementary material for: SurgUn: Exploiting Concept Identifiability in Diffusion Models for Gradient-Based Surgical Unlearning
Source: arXiv:2603.00975 source file (2026-12-01)
Supplement: Supplementary file 1 [file method_backbone_appendix.tex]

\begin{table}[!tbh]
\caption{
A summary of the unlearning methods and the corresponding models used in our experiments. Among these methods, ESD and SurgUn are the only approaches that generalize to both U-Net–based and DiT-based architectures. However, ESD shows substantially lower retention accuracy, as reported in Table \ref{tab: style_and_object}, whereas SurgUn maintains strong retention while remaining model-agnostic.
}
\label{tab: method_backbone}
\small
\begin{tabular}{|l|c|c|c|}
\hline
Method & U-Net (SD v1.5) & U-Net (SDXL) & DiT \\ \hline
ESD & \textcolor{green}{\cmark} & \textcolor{green}{\cmark} & \textcolor{green}{\cmark} \\ \hline
FMN & \textcolor{green}{\cmark}  & \textcolor{green}{\cmark}  & \textcolor{red}{\xmark} \\ \hline
UCE & \textcolor{green}{\cmark}  & \textcolor{red}{\xmark} & \textcolor{red}{\xmark}  \\ \hline
CA & \textcolor{green}{\cmark} & \textcolor{red}{\xmark}  &  \textcolor{red}{\xmark} \\ \hline
SalUN & \textcolor{green}{\cmark}  & \textcolor{red}{\xmark}  & \textcolor{red}{\xmark} \\ \hline
SEOT & \textcolor{green}{\cmark} & \textcolor{green}{\cmark}  & \textcolor{red}{\xmark} \\ \hline
SPM & \textcolor{green}{\cmark}  & \textcolor{red}{\xmark} &  \textcolor{red}{\xmark}\\ \hline
EDiff &\textcolor{green}{\cmark}  & \textcolor{red}{\xmark}  & \textcolor{red}{\xmark} \\ \hline
SHS & \textcolor{green}{\cmark} & \textcolor{red}{\xmark}  & \textcolor{red}{\xmark} \\ \hline
SAeUron & \textcolor{green}{\cmark}   & \textcolor{red}{\xmark}  & \textcolor{red}{\xmark} \\ \hline
SurgUn (Ours) & \textcolor{green}{\cmark} & \textcolor{green}{\cmark}  & \textcolor{green}{\cmark} \\ \hline
\end{tabular}
\end{table}
