# Supplementary material for: SurgUn: Exploiting Concept Identifiability in Diffusion Models for Gradient-Based Surgical Unlearning
Source: arXiv:2603.00975 source file (2026-12-01)
Supplement: Supplementary file 2 [file ip_sana.tex]

\begin{figure*}[!tbh]
    \centering
    \begin{subfigure}{0.4\textwidth}
        \centering
        \includegraphics[width=\linewidth]{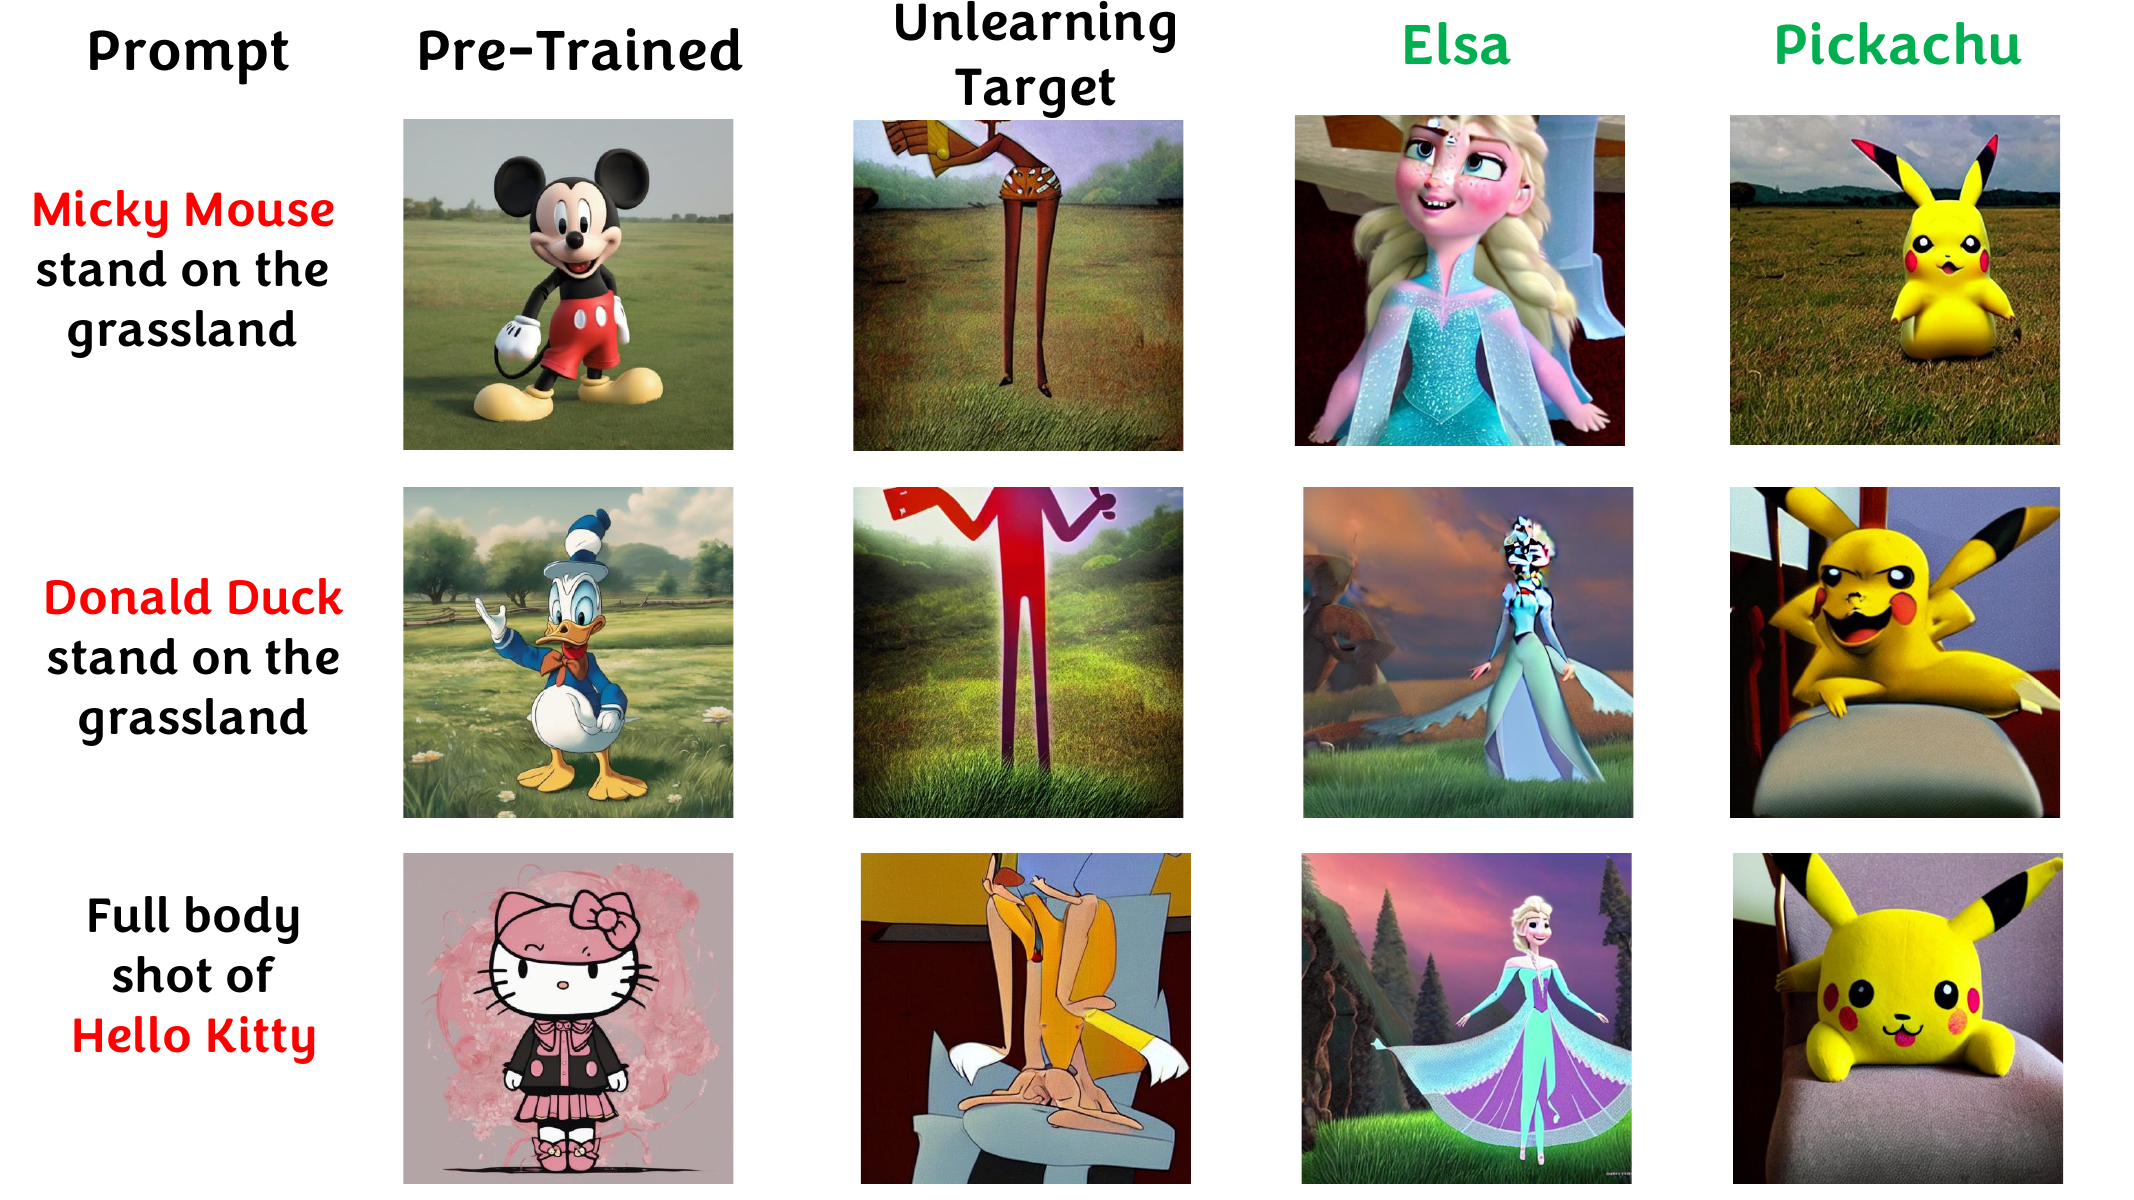}
        \caption{ACE}
    \end{subfigure}
    \hfill
        \begin{subfigure}{0.4\textwidth}
        \centering
        \includegraphics[width=\linewidth]{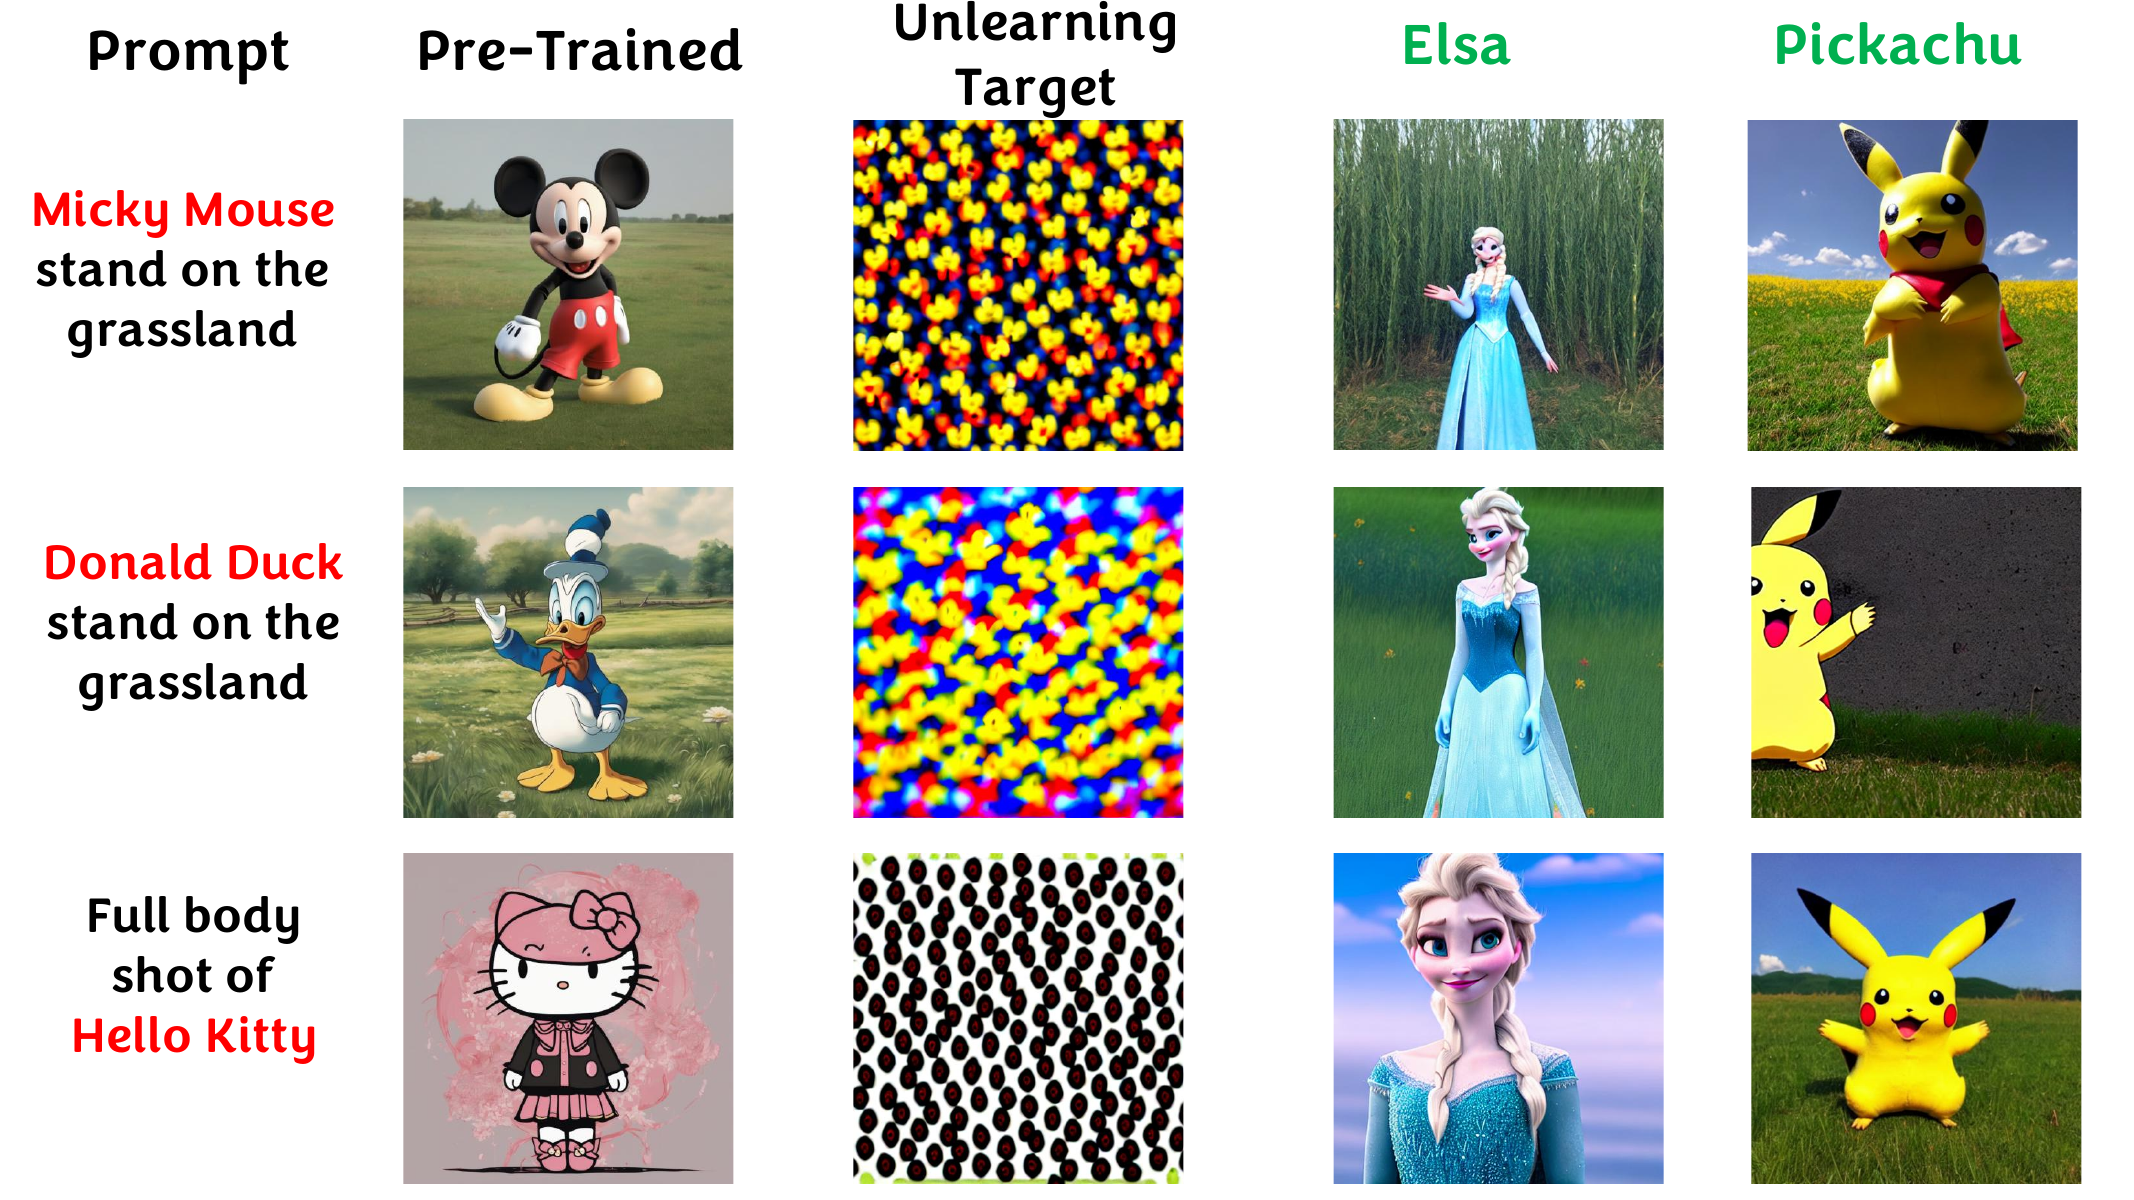}
        \caption{SurgUn (SDv1.5)}
    \end{subfigure}
        \begin{subfigure}{0.4\textwidth}
        \centering
        \includegraphics[width=\linewidth]{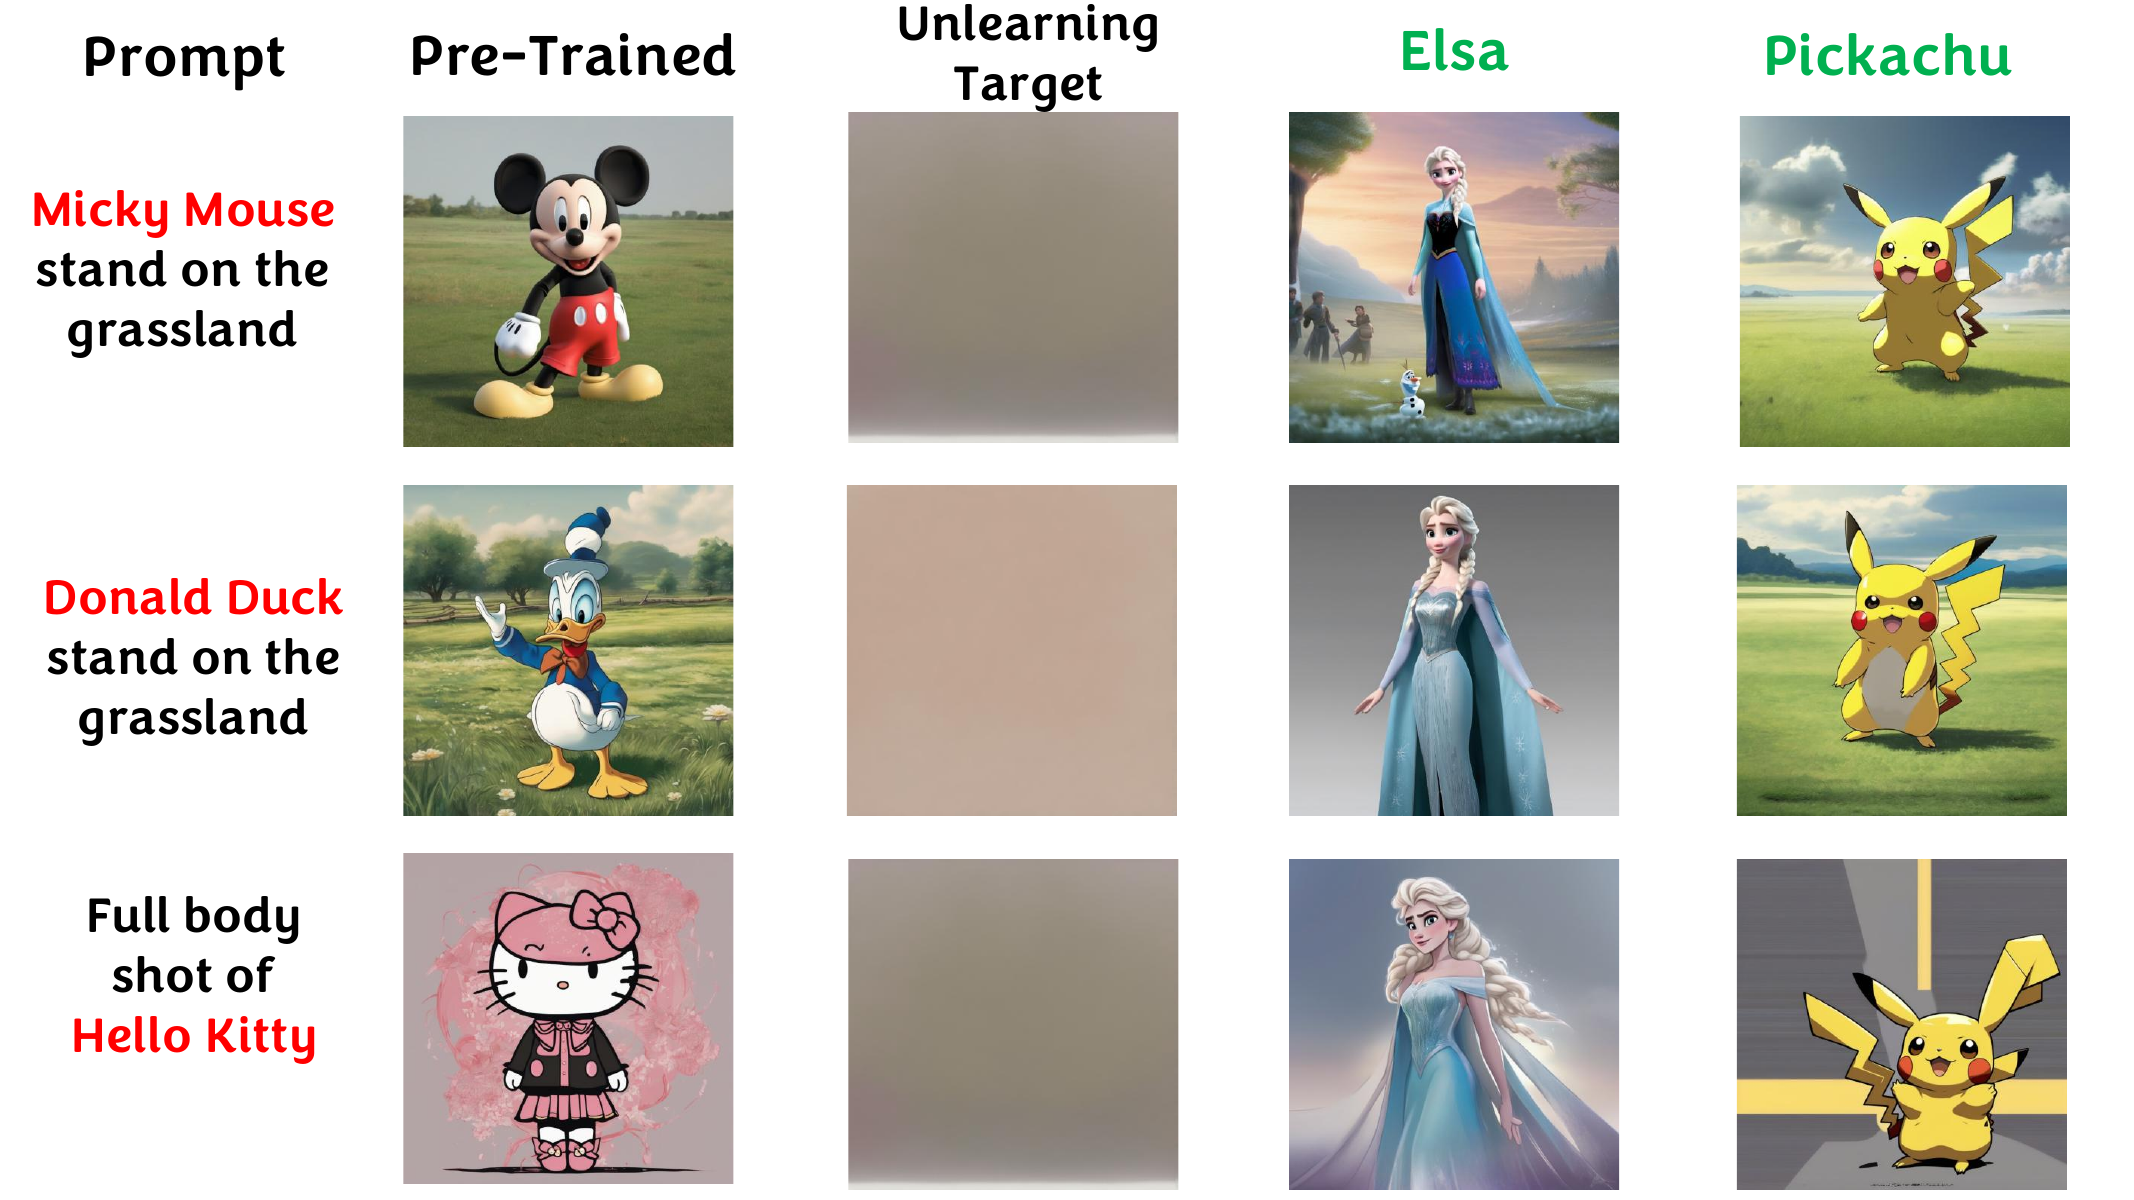}
        \caption{SurgUn (SDXL)}
    \end{subfigure}
    
    \begin{subfigure}{0.4\textwidth}
        \centering
        \includegraphics[width=\linewidth]{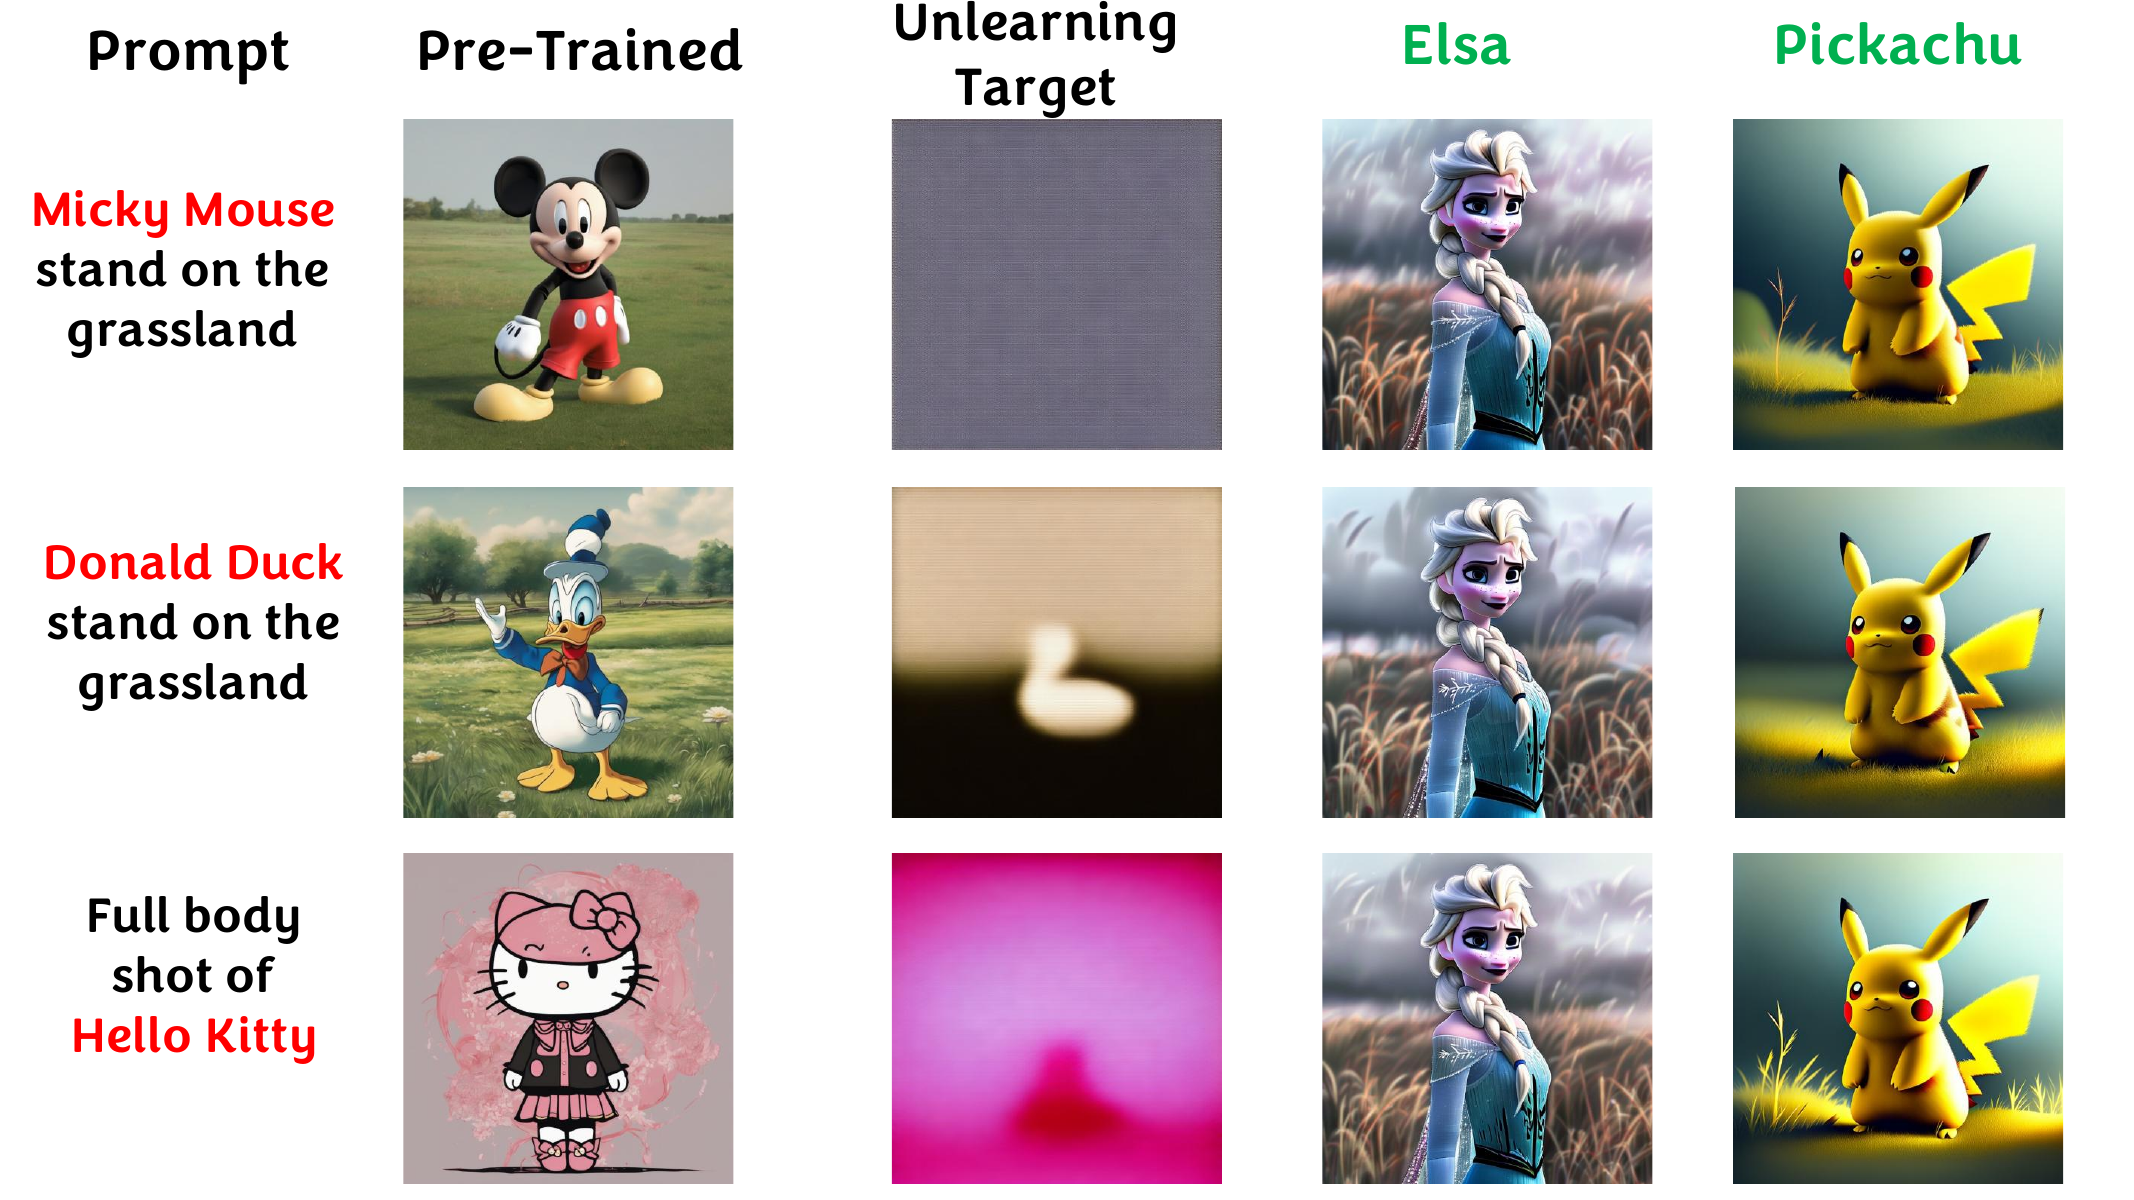}
        \caption{SurgUn (SANA)}
    \end{subfigure}
    \caption{Qualitative comparison of IP removal of ACE, SurgUn (SD v1.5), SurgUn (SDXL) and SurgUn (SANA). \textcolor{red!50}{Red} colour highlights the unlearning target while \textcolor{green!50}{Green} colour represent unrelated concept to evaluate retainability of model.}
\label{fig: ip_result_quali_appendix}
\end{figure*}
