# Supplementary material for: SurgUn: Exploiting Concept Identifiability in Diffusion Models for Gradient-Based Surgical Unlearning
Source: arXiv:2603.00975 source file (2026-12-01)
Supplement: Supplementary file 4 [file obj_unlearning_appendix.tex]

\begin{figure}[!tbh]
    \centering
    % \begin{subfigure}{0.65\textwidth}
    %     \centering
    %     \resizebox{\linewidth}{!}{\includegraphics[]{appendix/images/bear_object_unlearn.pdf}} % First image
    %     \caption{Unlearning Target: Bear}
    % \end{subfigure}
    % \vspace{10pt} % Space between images
    % \begin{subfigure}{0.65\textwidth}
    %     \centering
    %     \resizebox{\linewidth}{!}{\includegraphics[]{appendix/images/flower_object_unlearn.pdf}} % Second image
    %     \caption{Unlearning Target: Flower}
    % \end{subfigure}
    % \vspace{10pt} % Space between images
    \begin{subfigure}{0.5\textwidth}
        \centering
        \resizebox{\linewidth}{!}{\includegraphics[]{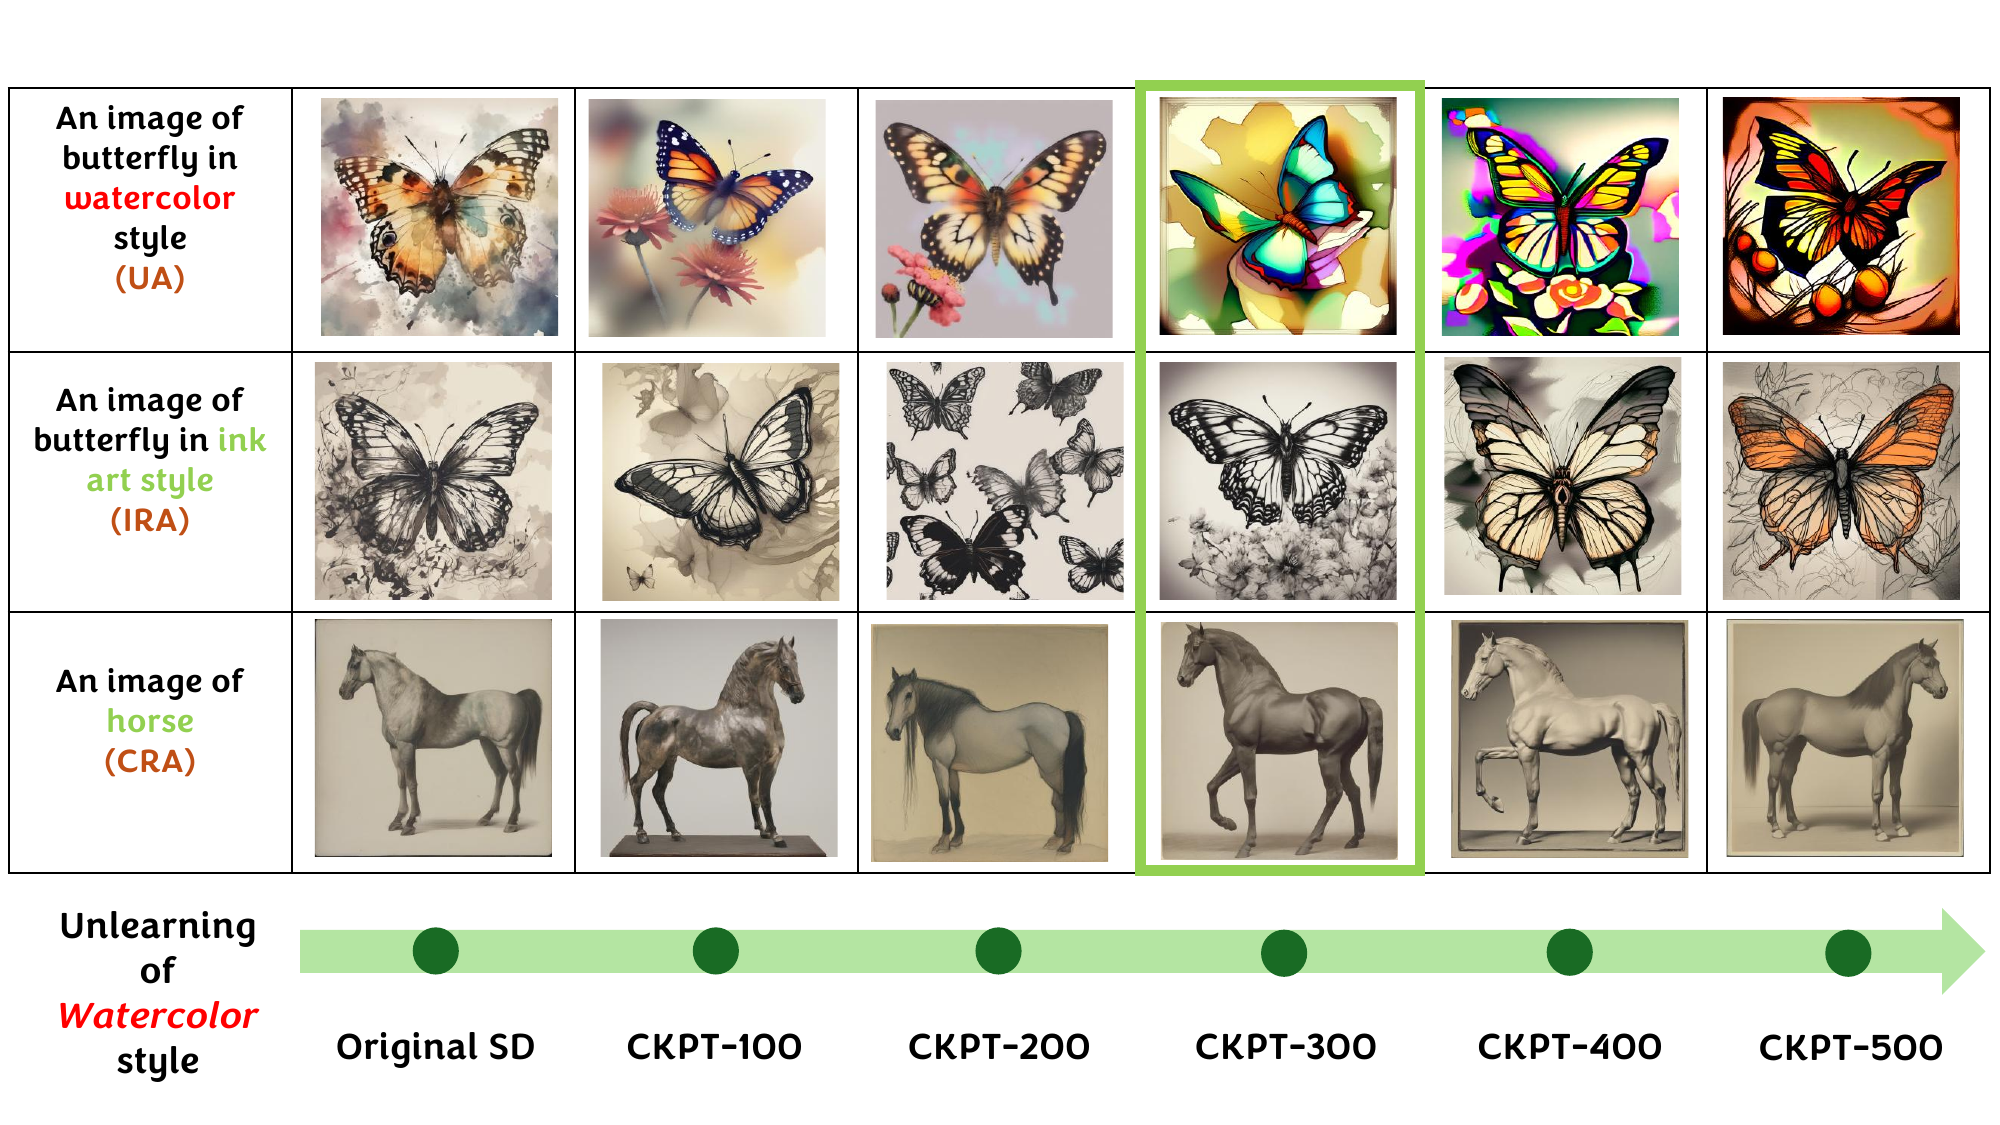}} % Second image
        \caption{Unlearning Target: Watercolor Style}
    \end{subfigure}
    \begin{subfigure}{0.5\textwidth}
        \centering
        \resizebox{\linewidth}{!}{\includegraphics[]{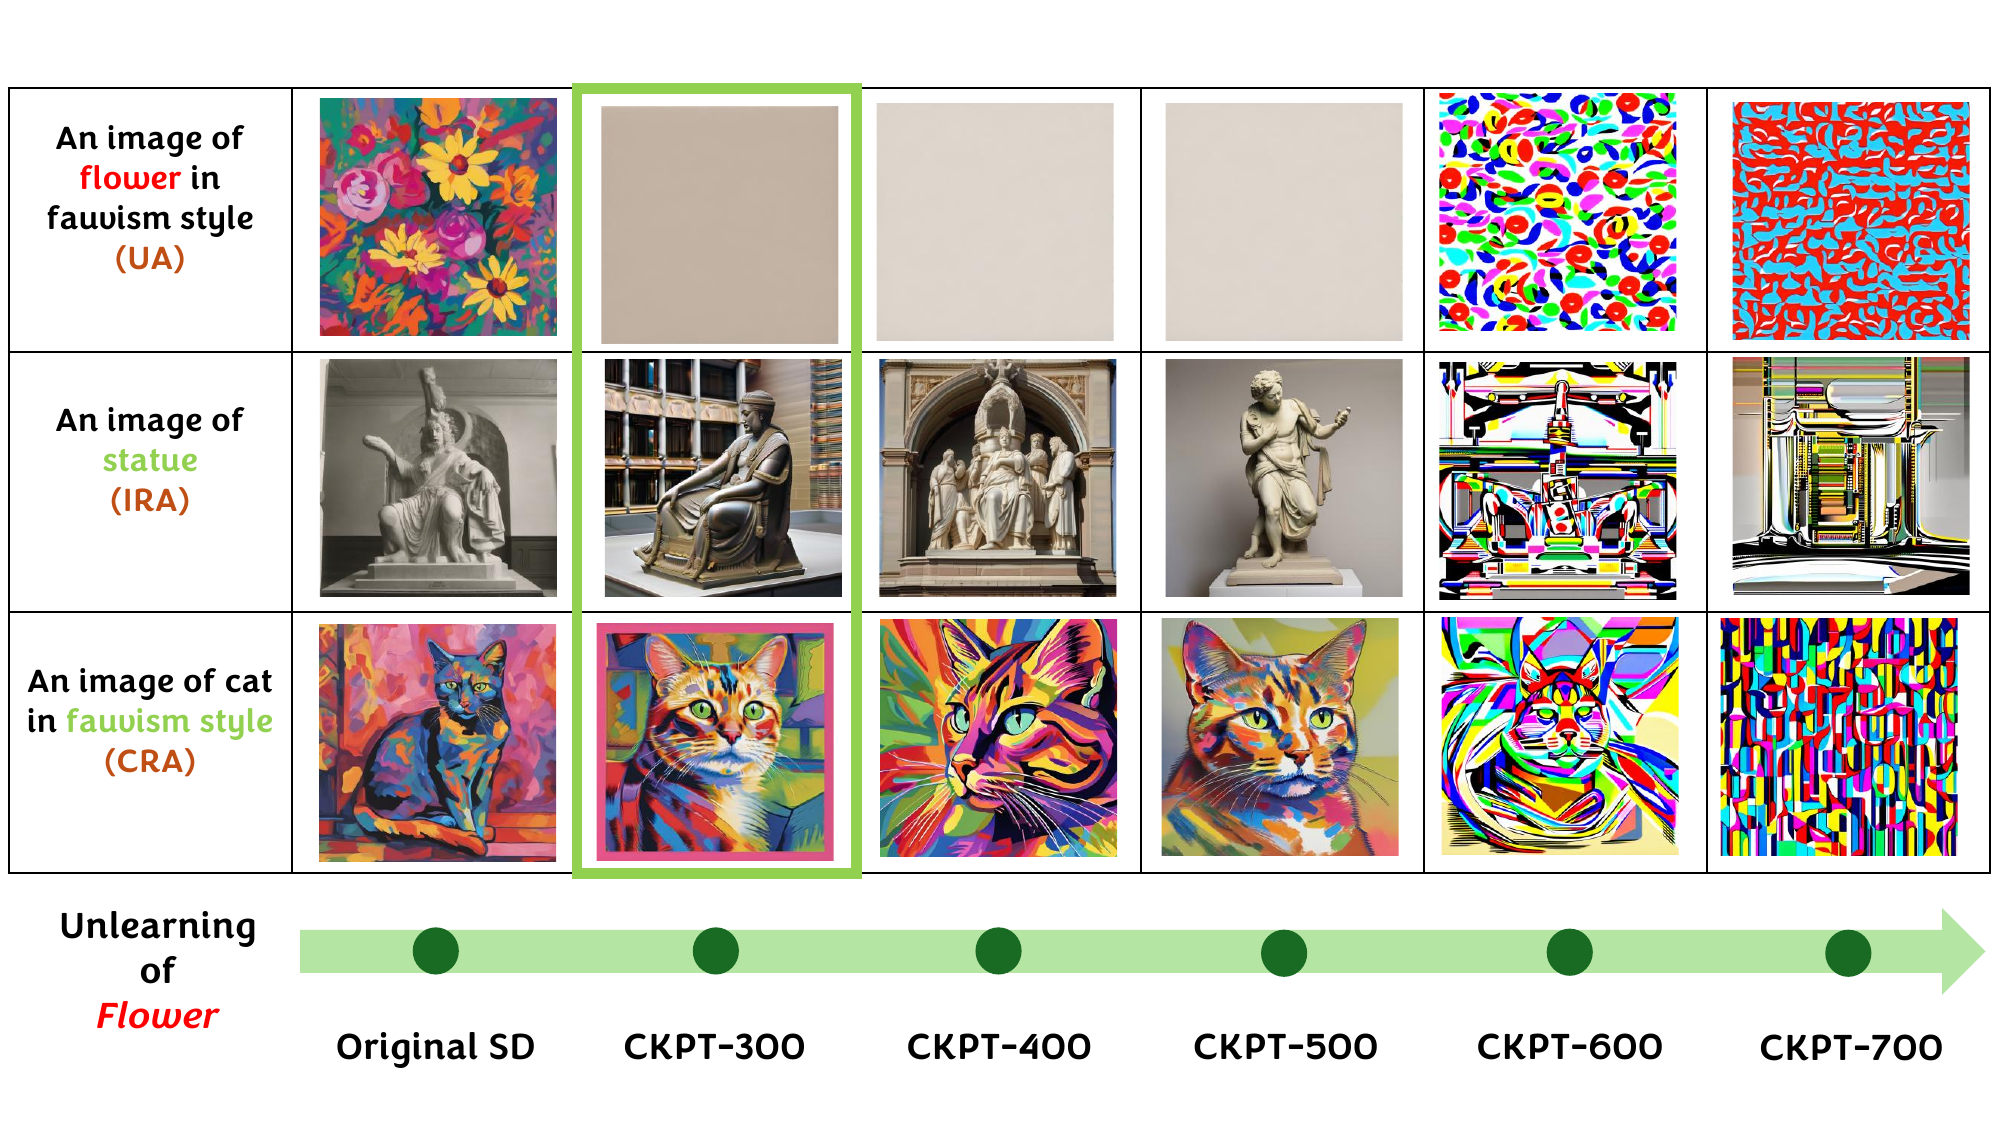}} % Third image
        \caption{Unlearning Target: Flower}
    \end{subfigure}
        \begin{subfigure}{0.5\textwidth}
        \centering
        \resizebox{\linewidth}{!}{\includegraphics[]{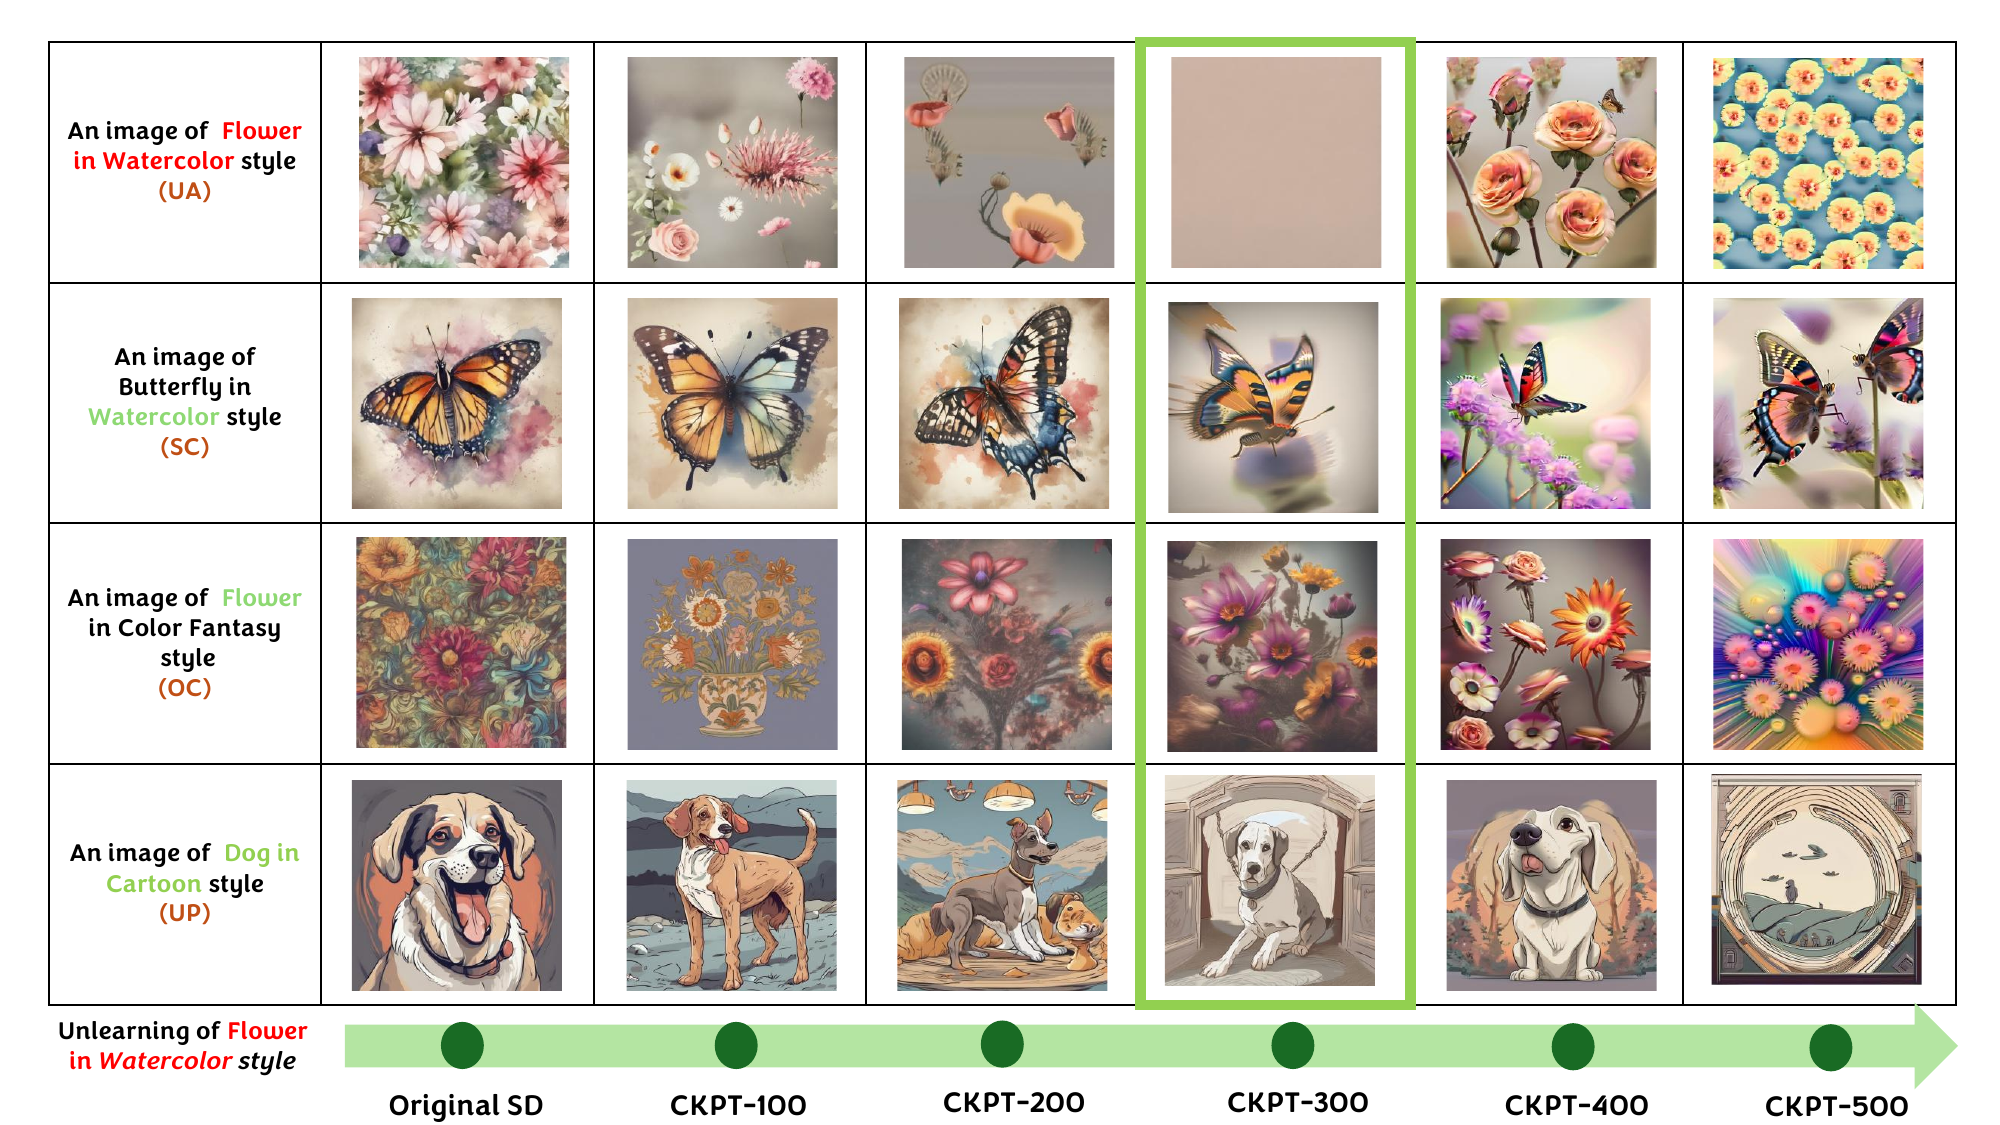}} % Third image
        \caption{Unlearning Target: Flower in Watercolor Style}
    \end{subfigure}
    \caption{Unlearning and retainability across checkpoints for the style, object, and combined unlearning tasks using SurgUn (SDXL). We highlight the best checkpoint for each target concept unlearning.}
    \label{fig: object_unlearn_1_appendix}
\end{figure}
