# Supplementary material for: SurgUn: Exploiting Concept Identifiability in Diffusion Models for Gradient-Based Surgical Unlearning
Source: arXiv:2603.00975 source file (2026-12-01)
Supplement: Supplementary file 6 [file sequential_appendix.tex]

% Please add the following required packages to your document preamble:
% \usepackage{multirow}
\begin{table}[t]
\caption{\textbf{Sequential unlearning}: Performance comparison of SalUN and SurgUn on the sequential unlearning of six styles. Each column represents a new unlearning request, denoted by $\mathcal{T}_i$
, where $\mathcal{T}_1$ is the oldest. The retaining accuracy (RA) is given by the average of IRA and CRA. We highlight the rebound effect with the orange color.}
\label{tab: continual_appendix}
\tiny{
% \resizebox{\linewidth}{!}{
\begin{tabular}{|cccccccc|}
\hline
\multicolumn{8}{|c|}{\textbf{Method: SalUn}} \\ \hline
\multicolumn{2}{|c|}{\multirow{2}{*}{\textbf{}}} & \textit{\textbf{$\mathcal{T}_1$}} & \textbf{$\mathcal{T}_1$$\sim$$\mathcal{T}_2$} & \textbf{$\mathcal{T}_1$$\sim$$\mathcal{T}_3$} & \textbf{$\mathcal{T}_1$$\sim$$\mathcal{T}_4$} & \textbf{$\mathcal{T}_1$$\sim$$\mathcal{T}_5$} & \textbf{$\mathcal{T}_1$$\sim$$\mathcal{T}_6$} \\ \cline{3-8}  
% \multicolumn{2}{|c|}{} & \multicolumn{6}{|c|}{\textbf{Unlearning Request}} \\ \hline
\multirow{6}{*}{\textbf{UA}} & \multicolumn{1}{c|}{\textbf{$\mathcal{T}_1$}} & \cellcolor{orange!50}{{84\%}} & \cellcolor{orange!50}{{79\%}} & \cellcolor{orange!50}{{78\%}} & \cellcolor{orange!50}{{65\%}} & \cellcolor{orange!50}{{67\%}} & \cellcolor{orange!50}{{64\%}}  \\
 & \multicolumn{1}{c|}{{$\mathcal{T}_2$}} & - & \cellcolor{orange!50}{{81.42\%}} & \cellcolor{orange!50}{{75\%}} & \cellcolor{orange!50}{{72\%}} & \cellcolor{orange!50}{{69\%}} & \cellcolor{orange!50}{{61\%}}  \\
 & \multicolumn{1}{c|}{{$\mathcal{T}_3$}} & - & - & \cellcolor{orange!50}90\% & \cellcolor{orange!50}85\% & \cellcolor{orange!50}84\% & \cellcolor{orange!50}87\%  \\
 & \multicolumn{1}{c|}{{$\mathcal{T}_4$}} & - & - & - & \cellcolor{orange!50}84\% & \cellcolor{orange!50}86\% & \cellcolor{orange!50}81\% \\
 & \multicolumn{1}{c|}{{$\mathcal{T}_5$}} & - & - & - & - & 79\% & 81\%  \\
 & \multicolumn{1}{c|}{{$\mathcal{T}_6$}} & - & - & - & - & - & 89\% \\ \hline
\multicolumn{2}{|c|}{\textbf{RA}} & 85.43\% & 80.32\% & 71.42\% & 65.41\% & 63.24\% & 60.19\% \\ \hline
\multicolumn{8}{|c|}{\textbf{Method: SurgUn}} \\ \hline
\multicolumn{2}{|c|}{\multirow{2}{*}{\textbf{}}} & \textit{\textbf{$\mathcal{T}_1$}} & \textbf{$\mathcal{T}_1$$\sim$$\mathcal{T}_2$} & \textbf{$\mathcal{T}_1$$\sim$$\mathcal{T}_3$} & \textbf{$\mathcal{T}_1$$\sim$$\mathcal{T}_4$} & \textbf{$\mathcal{T}_1$$\sim$$\mathcal{T}_5$} & \textbf{$\mathcal{T}_1$$\sim$$\mathcal{T}_6$} \\ \cline{3-8}  
% \multicolumn{2}{|c|}{} & \multicolumn{6}{|c|}{\textbf{Unlearning Request}} \\ \hline

\multirow{6}{*}{\textbf{UA}} & \multicolumn{1}{c|}{\textbf{$\mathcal{T}_1$}} & 100\% & 100\% & 100\% & 100\% & 100\% & 100\% \\
 & \multicolumn{1}{c|}{\textbf{$\mathcal{T}_2$}} & - & \cellcolor{orange!50}100\% & \cellcolor{orange!50}100\% & \cellcolor{orange!50}82\% & \cellcolor{orange!50}75\% & \cellcolor{orange!50}78\% \\
 & \multicolumn{1}{c|}{\textbf{$\mathcal{T}_3$}} & - & - & 100\% & 100\% & 100\% & 100\%  \\
 & \multicolumn{1}{c|}{\textbf{$\mathcal{T}_4$}} & - & - & - & 100\% & 100\% & 100\%  \\
 & \multicolumn{1}{c|}{\textbf{$\mathcal{T}_5$}} & - & - & - & - & 100\% & 100\%  \\
 & \multicolumn{1}{c|}{\textbf{$\mathcal{T}_6$}} & - & - & - & - & - & 100\% &   \hline
\multicolumn{2}{|c|}{\textbf{RA}} & 85\% & 78\% & 72\% & 65\% & 64.5\% & 65\% \\ \hline
\end{tabular}
}
% }
\end{table}
