# Supplementary material for: SurgUn: Exploiting Concept Identifiability in Diffusion Models for Gradient-Based Surgical Unlearning
Source: arXiv:2603.00975 source file (2026-12-01)
Supplement: Supplementary file 9 [file adversarial_attack.tex]

\begin{table}[!tbh]
\caption{\textbf{Adversarial Attack Success Rates (ASR)}. The best two results are highlighted with \textcolor{green!50}{green} and \textcolor{blue!50}{blue} respectively. The worst results are highlighted with \textcolor{red!50}{red}. Lower ASR suggest high resistance to adversarial attacks.}
\label{table: appendix_adv_attack}
\centering
\resizebox{\linewidth}{!}{\begin{tabular}{lcccccccc}
\toprule
Concept & K & ESD & CA & FMN & SalUn & \multicolumn{3}{c}{SurgUn} \\
\cmidrule(lr){7-9}
 &  &  &  &  &  & SD v1.5 & SDXL & SANA \\
\midrule
\multirow{3}{*}{Nudity} & 77 & 19.40\% & \cellcolor{red!25}82.32\% & 61.22\% & \cellcolor{green!25}0.00\% & \cellcolor{green!25}0.0\% & 17.94\% & 14.32\% \\
 & 38 & 25.47\% & \cellcolor{red!25}87.58\% & 67.58\% & \cellcolor{green!25}0.0\% & \cellcolor{green!25}0.0\% & 18.11\% & 10.89\% \\
 & 16 & 28.39\% & \cellcolor{red!25}85.46\% & 68.42\% & \cellcolor{green!25}0.0\% & \cellcolor{green!25}0.0\% & 11.02\% & 9.22\% \\
\midrule
\multirow{3}{*}{Violence} & 77 & 54.00\% & \cellcolor{red!25}97.60\% & 79.60\% & 24.81\% & \cellcolor{blue!25}10.21\% & 13.81\% & \cellcolor{green!25}9.09\% \\
 & 38 & 46.40\% & \cellcolor{red!25}95.20\% & 82.40\% & 22.48\% & \cellcolor{green!25}12.32\% & 18.04\% & \cellcolor{blue!25}13.44\% \\
 & 16 & 48.80\% & \cellcolor{red!25}88.00\% & 76.00\% & 23.20\% & \cellcolor{green!25}5.54\% & 12.33\% & \cellcolor{blue!25}10.01\% \\
\bottomrule
\end{tabular}}
\end{table}
