# Supplementary material for: SurgUn: Exploiting Concept Identifiability in Diffusion Models for Gradient-Based Surgical Unlearning
Source: arXiv:2603.00975 source file (2026-12-01)
Supplement: Supplementary file 10 [file selective_test.tex]

\begin{table}[t]
\centering
\scriptsize
\setlength{\tabcolsep}{4pt}
\renewcommand{\arraystretch}{1.1}

\caption{
\textbf{Selective concept unlearning under compositional prompts.}
We evaluate Dog unlearning across four diffusion architectures
using prompts containing the target (Dog) alongside non-target
objects. We generate 10 images per model and report the
average CLIP similarity scores before and after unlearning.
Lower target alignment indicates successful suppression,
while higher non-target alignment indicates better preservation.
}
\label{tab:compositional_clip}

\resizebox{\columnwidth}{!}{%
\begin{tabular}{lcc}
\toprule

\textbf{Model}
& \textbf{Target CLIP (Before/After)}
& \textbf{Non-target CLIP (Before/After)} \\

\midrule

SD v1.5
& 33.09 / 25.11
& 34.71 / 23.88 \\

SDXL
& 32.76 / 25.65
& 33.44 / 30.55 \\

SANA 1.5
& 33.20 / 22.86
& 32.19 / 31.45 \\

SD3.5
& 34.77 / 23.80
& 34.60 / 32.79 \\

\bottomrule
\end{tabular}%
}

\end{table}
